# Supplementary material for: Multi-modal Pose Diffuser: A Multimodal Generative Conditional Pose Prior
Source: arXiv:2410.14540 source file (2024-10-18)
Supplement: Supplementary file 1 [file 06_supp.tex]

\title{Supplemental Material: Multi-modal Pose Diffuser: A Multimodal Generative Conditional Pose Prior} 
\maketitle

\section{Architecture}
The architecture we use for the context encoder $\mathcal{F}$ is a text-prompt based 2D key-point estimator CLAMP\cite{zhang2023clamp}. CLAMP uses a fixed set of text prompts at inference and for our use case we use the MSCOCO\cite{lin2014microsoft} joint names. Given an image input we utilize the feature maps provided by the image encoder and sample feature vectors based off the estimated 2D key-points. This gives us $c_\mathcal{I}$ and depending on if a text description is provided we pass both $c_\mathcal{I}$ and $c_\mathcal{T}$ to the context encoder which outputs a fixed-length context sequence $c\in \mathcal{R}^{21 \times D} $ where 21 is the number of SMPL joints we are modeling (we are ignoring the global-orientation and the hand joints). 
\begin{figure}
    \centering
    \includegraphics[width=0.95\linewidth]{sections//figures/Context Model.png}
    \caption{Overview of the condition encoder $\mathcal{F}$ in \cref{fig:diffusion_arch}. For the condition encoder we leverage a pre-trained \cite{zhang2023clamp} trained for human pose estimation.}
    \label{fig:context_model}
\end{figure}
\section{Timestep Choices}
It has been widely observed\cite{karras2022elucidating, choi2022perception} that the earlier timesteps in the sampling process generally introduce larger changes when transitioning between timestep $t$ and $t-1$. As $t$ approaches 0 the changes become much smaller in magnitude and for our purposes are far more useful when $\mathcal{G}$ is used as a prior. The timestep choice was empirically chosen and while not an exhaustive search we found that $t=50$ resulted in strong performance. Investigating a more principled selection process for $t$ is left to future work. 

\newpage
\section{Additional Qualitative Results- Pose Estimation}
Here we provide larger versions of images shown in \cref{fig:ehf} and \cref{fig:qual_hmr} of the main paper. Note that our method depends on the OpenPose\cite{8765346} key-points and inaccurate key-points may lead to incorrect 3D poses.
\begin{figure}
\centering
\begin{tikzpicture}[picture format/.style={inner sep=0pt,}]

  \node[picture format]                   (A1)               {\includegraphics[trim=350 0 350 0,clip, width=1.7in]{sections/figures/hmr_images/ours/ehf_gt/01_img.png}};
  % \node[picture format,anchor=north]      (B1) at (A1.south) {\includegraphics[trim=350 0 350 0,clip, width=1.5in]{sections/figures/hmr_images/ours/ehf_gt/05_img.png}};
  %   \node[picture format,anchor=north]      (C1) at (B1.south) {\includegraphics[trim=350 0 350 0,clip, width=1.5in]{sections/figures/hmr_images/ours/ehf_gt/09_img.png}};

  \node[picture format, anchor=north west] (A2) at (A1.north east){\includegraphics[trim=350 0 350 0,clip, width=1.7in]{sections/figures/hmr_images/ours/01_img_[82.61552066640219]_[128.095022308605]mesh_fit.png}};
  % \node[picture format,anchor=north]      (B2) at (A2.south) {\includegraphics[trim=350 0 350 0,clip, width=1.5in]{sections/figures/hmr_images/ours/05_img_[68.96444262276147]_[76.62396137146361]mesh_fit.png}};
  %   \node[picture format,anchor=north]      (C2) at (B2.south) {\includegraphics[trim=350 0 350 0,clip, width=1.5in]{sections/figures/hmr_images/ours/09_img_[53.447338233828674]_[71.96820752530422]mesh_fit.png}};

  \node[picture format,anchor=north] (A3) at (A1.south) {\includegraphics[trim=350 0 350 0,clip, width=1.7in]{sections/figures/hmr_images/dposer/01_img_mesh_fit.png}};
  % \node[picture format,anchor=north]      (B3) at (A3.south)      {\includegraphics[trim=350 0 350 0,clip, width=1.5in]{sections/figures/hmr_images/dposer/05_img_mesh_fit.png}};
  %   \node[picture format,anchor=north]      (C3) at (B3.south)      {\includegraphics[trim=350 0 350 0,clip, width=1.5in]{sections/figures/hmr_images/dposer/09_img_mesh_fit.png}};

  \node[picture format,anchor=north west] (A4) at (A3.north east) {\includegraphics[trim=350 0 350 0,clip, width=1.7in]{sections/figures/hmr_images/posendf/01_img_[210.20784889717345]_[267.5707375239675]_mesh_fit.png}};
  % \node[picture format,anchor=north]      (B4) at (A4.south)      {\includegraphics[trim=350 0 350 0,clip, width=1.5in]{sections/figures/hmr_images/posendf/05_img_[151.21564345207153]_[277.34793353709813]_mesh_fit.png}};
  %   \node[picture format,anchor=north]      (C4) at (B4.south)      {\includegraphics[trim=350 0 350 0,clip, width=1.5in]{sections/figures/hmr_images/posendf/09_img_[74.66004911795598]_[151.95715054949346]_mesh_fit.png}};

  %% Captions
 \node[anchor=south] (D1) at (A1.north) {\bfseries Original};
\node[anchor=south] (D2) at (A2.north) {\bfseries \method{} (Ours)};
  \node[anchor=north] (D3) at (A3.south) {\bfseries DPoser\cite{lu2023dposer}};
  \node[anchor=north] (D4) at (A4.south) {\bfseries PoseNDF\cite{tiwari2022pose}};

\end{tikzpicture}
\caption{Larger EHF images (1)}
\label{fig:ehf_larger}
\end{figure}

\begin{figure}
\centering
\begin{tikzpicture}[picture format/.style={inner sep=0pt,}]

  \node[picture format]                   (A1)               {\includegraphics[trim=350 0 350 0,clip, width=1.7in]{sections/figures/hmr_images/ours/ehf_gt/05_img.png}};
  % \node[picture format,anchor=north]      (B1) at (A1.south) {\includegraphics[trim=350 0 350 0,clip, width=1.5in]{sections/figures/hmr_images/ours/ehf_gt/05_img.png}};
  %   \node[picture format,anchor=north]      (C1) at (B1.south) {\includegraphics[trim=350 0 350 0,clip, width=1.5in]{sections/figures/hmr_images/ours/ehf_gt/09_img.png}};

  \node[picture format, anchor=north west] (A2) at (A1.north east){\includegraphics[trim=350 0 350 0,clip, width=1.7in]{sections/figures/hmr_images/ours/05_img_[68.96444262276147]_[76.62396137146361]mesh_fit.png}};
  % \node[picture format,anchor=north]      (B2) at (A2.south) {\includegraphics[trim=350 0 350 0,clip, width=1.5in]{sections/figures/hmr_images/ours/05_img_[68.96444262276147]_[76.62396137146361]mesh_fit.png}};
  %   \node[picture format,anchor=north]      (C2) at (B2.south) {\includegraphics[trim=350 0 350 0,clip, width=1.5in]{sections/figures/hmr_images/ours/09_img_[53.447338233828674]_[71.96820752530422]mesh_fit.png}};

  \node[picture format,anchor=north] (A3) at (A1.south) {\includegraphics[trim=350 0 350 0,clip, width=1.7in]{sections/figures/hmr_images/dposer/05_img_mesh_fit.png}};
  % \node[picture format,anchor=north]      (B3) at (A3.south)      {\includegraphics[trim=350 0 350 0,clip, width=1.5in]{sections/figures/hmr_images/dposer/05_img_mesh_fit.png}};
  %   \node[picture format,anchor=north]      (C3) at (B3.south)      {\includegraphics[trim=350 0 350 0,clip, width=1.5in]{sections/figures/hmr_images/dposer/09_img_mesh_fit.png}};

  \node[picture format,anchor=north west] (A4) at (A3.north east) {\includegraphics[trim=350 0 350 0,clip, width=1.7in]{sections/figures/hmr_images/posendf/05_img_[151.21564345207153]_[277.34793353709813]_mesh_fit.png}};
  % \node[picture format,anchor=north]      (B4) at (A4.south)      {\includegraphics[trim=350 0 350 0,clip, width=1.5in]{sections/figures/hmr_images/posendf/05_img_[151.21564345207153]_[277.34793353709813]_mesh_fit.png}};
  %   \node[picture format,anchor=north]      (C4) at (B4.south)      {\includegraphics[trim=350 0 350 0,clip, width=1.5in]{sections/figures/hmr_images/posendf/09_img_[74.66004911795598]_[151.95715054949346]_mesh_fit.png}};

  %% Captions
 \node[anchor=south] (D1) at (A1.north) {\bfseries Original};
\node[anchor=south] (D2) at (A2.north) {\bfseries \method{} (Ours)};
  \node[anchor=north] (D3) at (A3.south) {\bfseries DPoser\cite{lu2023dposer}};
  \node[anchor=north] (D4) at (A4.south) {\bfseries PoseNDF\cite{tiwari2022pose}};

\end{tikzpicture}
\caption{Larger EHF images (2)}
\label{fig:ehf_larger2}
\end{figure}

\begin{figure}
\centering
\begin{tikzpicture}[picture format/.style={inner sep=0pt,}]

  \node[picture format]                   (A1)               {\includegraphics[trim=350 0 350 0,clip, width=1.7in]{sections/figures/hmr_images/ours/ehf_gt/09_img.png}};
  % \node[picture format,anchor=north]      (B1) at (A1.south) {\includegraphics[trim=350 0 350 0,clip, width=1.5in]{sections/figures/hmr_images/ours/ehf_gt/05_img.png}};
  %   \node[picture format,anchor=north]      (C1) at (B1.south) {\includegraphics[trim=350 0 350 0,clip, width=1.5in]{sections/figures/hmr_images/ours/ehf_gt/09_img.png}};

  \node[picture format, anchor=north west] (A2) at (A1.north east){\includegraphics[trim=350 0 350 0,clip, width=1.7in]{sections/figures/hmr_images/ours/09_img_[53.447338233828674]_[71.96820752530422]mesh_fit.png}};
  % \node[picture format,anchor=north]      (B2) at (A2.south) {\includegraphics[trim=350 0 350 0,clip, width=1.5in]{sections/figures/hmr_images/ours/05_img_[68.96444262276147]_[76.62396137146361]mesh_fit.png}};
  %   \node[picture format,anchor=north]      (C2) at (B2.south) {\includegraphics[trim=350 0 350 0,clip, width=1.5in]{sections/figures/hmr_images/ours/09_img_[53.447338233828674]_[71.96820752530422]mesh_fit.png}};

  \node[picture format,anchor=north] (A3) at (A1.south) {\includegraphics[trim=350 0 350 0,clip, width=1.7in]{sections/figures/hmr_images/dposer/09_img_mesh_fit.png}};
  % \node[picture format,anchor=north]      (B3) at (A3.south)      {\includegraphics[trim=350 0 350 0,clip, width=1.5in]{sections/figures/hmr_images/dposer/05_img_mesh_fit.png}};
  %   \node[picture format,anchor=north]      (C3) at (B3.south)      {\includegraphics[trim=350 0 350 0,clip, width=1.5in]{sections/figures/hmr_images/dposer/09_img_mesh_fit.png}};

  \node[picture format,anchor=north west] (A4) at (A3.north east) {\includegraphics[trim=350 0 350 0,clip, width=1.7in]{sections/figures/hmr_images/posendf/09_img_[74.66004911795598]_[151.95715054949346]_mesh_fit.png}};
  % \node[picture format,anchor=north]      (B4) at (A4.south)      {\includegraphics[trim=350 0 350 0,clip, width=1.5in]{sections/figures/hmr_images/posendf/05_img_[151.21564345207153]_[277.34793353709813]_mesh_fit.png}};
  %   \node[picture format,anchor=north]      (C4) at (B4.south)      {\includegraphics[trim=350 0 350 0,clip, width=1.5in]{sections/figures/hmr_images/posendf/09_img_[74.66004911795598]_[151.95715054949346]_mesh_fit.png}};

  %% Captions
 \node[anchor=south] (D1) at (A1.north) {\bfseries Original};
\node[anchor=south] (D2) at (A2.north) {\bfseries \method{} (Ours)};
  \node[anchor=north] (D3) at (A3.south) {\bfseries DPoser\cite{lu2023dposer}};
  \node[anchor=north] (D4) at (A4.south) {\bfseries PoseNDF\cite{tiwari2022pose}};

\end{tikzpicture}
\caption{Larger EHF images (3)}
\label{fig:ehf_larger2}
\end{figure}

\begin{figure}
\centering
\begin{tikzpicture}[picture format/.style={inner sep=1pt, outer sep=0pt}]

  \node[picture format]                   (A1)               {\includegraphics[trim=350 0 350 0,clip, width=2.0in]{sections/figures/hmr_images/ours/ehf_gt/18_img.png}};
  
  \node[picture format,anchor=north west]      (B1) at (A1.north east) {\includegraphics[trim=350 0 350 0,clip, width=2.0in]{sections/figures/hmr_images/ours/18_img_[74.1666871091886]_[121.5710905741555]mesh_fit.png}};
\node[anchor=south] (C1) at (A1.north) {\bfseries Original};
\node[anchor=south] (C2) at (B1.north) {\bfseries \method{}(Ours)};

  \node[picture format, anchor=north] (A2) at (A1.south)     {\includegraphics[trim=300 450 200 300,clip, width=2.0in]{sections/figures/hmr_images/3dpw_orig/image_00210.jpg}};
  
  \node[picture format,anchor=north west]      (B2) at (A2.north east) {\includegraphics[trim=300 450 200 300,clip, width=2.0in]{sections/figures/hmr_images/3dpw/image_00210_mesh_fit.png}};

  % \node[picture format,anchor=north]      (B2) at (A2.south)      {\includegraphics[trim=225 10 850 10,clip, width=.9in]{sections/figures/hmr_images/3dpw/image_00325_mesh_fit.png}};
  %   \node[picture format,anchor=north]      (C2) at (B2.south)      {\includegraphics[trim=140 200 500 250,clip, width=.4in]{sections/figures/hmr_images/3dpw/image_01297.png}};
  %     \node[picture format,anchor=north]      (D2) at (C2.south)      {\includegraphics[trim=350 10 950 10,clip,width=.9in]{sections/figures/hmr_images/3dpw/image_01108_mesh_fit.png}};

  % \node[picture format,anchor=north west] (A3) at (A2.north east) {\includegraphics[trim=140 50 400 60,clip,width=.60in]{sections/figures/hmr_images/coco/COCO_train2014_000000031335_mesh_fit.png}};
  % \node[picture format,anchor=north]      (B3) at (A3.south)      {\includegraphics[trim=0 90 200 100,clip,width=.75in]{sections/figures/hmr_images/coco/COCO_train2014_000000273665_mesh_fit.png}};
  %   \node[picture format,anchor=north]      (C3) at (B3.south)      {\includegraphics[trim=400 0 0 0,clip,width=.65in]{sections/figures/hmr_images/coco/COCO_train2014_000000175669_mesh_fit.png}};
  %     \node[picture format,anchor=north]      (D3) at (C3.south)      {\includegraphics[trim=100 100 400 100,clip,width=0.7in]{sections/figures/hmr_images/coco/COCO_train2014_000000525169_mesh_fit.png}};

  %% Captions

  % \node[anchor=south] (E2) at (A2.north) {\bfseries 3DPW\cite{vonMarcard2018}};
  % \node[anchor=south] (E3) at (A3.north) {\bfseries COCO\cite{lin2014microsoft}};

\end{tikzpicture}
\caption{Qualitative Results from \method{} for 3D pose estimation across the EHF\cite{SMPL-X:2019}, 3DPW\cite{vonMarcard2018}, and COCO\cite{lin2014microsoft} Original vs Predicted} 
\label{fig:qual_hmr_vs_ori_1}
\end{figure}

\begin{figure}
\centering
\begin{tikzpicture}[picture format/.style={inner sep=1pt, outer sep=0pt}]

  \node[picture format]                   (A1)               {\includegraphics[trim=225 10 850 10,clip, width=2.0in]{sections/figures/hmr_images/3dpw_orig/image_00325.jpg}};
  
  \node[picture format,anchor=north west]      (B1) at (A1.north east)  {\includegraphics[trim=225 10 850 10,clip, width=2.0in]{sections/figures/hmr_images/3dpw/image_00325_mesh_fit.png}};
\node[anchor=south] (C1) at (A1.north) {\bfseries Original};
\node[anchor=south] (C2) at (B1.north) {\bfseries \method{}(Ours)};

  \node[picture format, anchor=north] (A2) at (A1.south)     {\includegraphics[trim=140 250 500 350,clip, width=1.5in]{sections/figures/hmr_images/3dpw_orig/image_01297.jpg}};
  
  \node[picture format,anchor=north west]      (B2) at (A2.north east) {\includegraphics[trim=140 250 500 350,clip, width=1.5in]{sections/figures/hmr_images/3dpw/image_01297.png}};

  % \node[picture format,anchor=north]      (B2) at (A2.south)      {\includegraphics[trim=225 10 850 10,clip, width=.9in]{sections/figures/hmr_images/3dpw/image_00325_mesh_fit.png}};
  %   \node[picture format,anchor=north]      (C2) at (B2.south)      {\includegraphics[trim=140 200 500 250,clip, width=.4in]{sections/figures/hmr_images/3dpw/image_01297.png}};
  %     \node[picture format,anchor=north]      (D2) at (C2.south)      {\includegraphics[trim=350 10 950 10,clip,width=.9in]{sections/figures/hmr_images/3dpw/image_01108_mesh_fit.png}};

  % \node[picture format,anchor=north west] (A3) at (A2.north east) {\includegraphics[trim=140 50 400 60,clip,width=.60in]{sections/figures/hmr_images/coco/COCO_train2014_000000031335_mesh_fit.png}};
  % \node[picture format,anchor=north]      (B3) at (A3.south)      {\includegraphics[trim=0 90 200 100,clip,width=.75in]{sections/figures/hmr_images/coco/COCO_train2014_000000273665_mesh_fit.png}};
  %   \node[picture format,anchor=north]      (C3) at (B3.south)      {\includegraphics[trim=400 0 0 0,clip,width=.65in]{sections/figures/hmr_images/coco/COCO_train2014_000000175669_mesh_fit.png}};
  %     \node[picture format,anchor=north]      (D3) at (C3.south)      {\includegraphics[trim=100 100 400 100,clip,width=0.7in]{sections/figures/hmr_images/coco/COCO_train2014_000000525169_mesh_fit.png}};

  %% Captions

  % \node[anchor=south] (E2) at (A2.north) {\bfseries 3DPW\cite{vonMarcard2018}};
  % \node[anchor=south] (E3) at (A3.north) {\bfseries COCO\cite{lin2014microsoft}};

\end{tikzpicture}
\caption{Qualitative Results from \method{} for 3D pose estimation across the EHF\cite{SMPL-X:2019}, 3DPW\cite{vonMarcard2018}, and COCO\cite{lin2014microsoft} Original vs Predicted (2)} 
\label{fig:qual_hmr_vs_ori_1}
\end{figure}

\begin{figure}
\centering
\begin{tikzpicture}[picture format/.style={inner sep=1pt, outer sep=0pt}]

  \node[picture format]                   (A1)               {\includegraphics[trim=350 10 950 10,clip,width=1.5in]{sections/figures/hmr_images/3dpw_orig/image_01108.jpg}};
  
  \node[picture format,anchor=north west]      (B1) at (A1.north east)  {\includegraphics[trim=350 10 950 10,clip,width=1.5in]{sections/figures/hmr_images/3dpw/image_01108_mesh_fit.png}};
\node[anchor=south] (C1) at (A1.north) {\bfseries Original};
\node[anchor=south] (C2) at (B1.north) {\bfseries \method{}(Ours)};

  \node[picture format, anchor=north] (A2) at (A1.south)     {\includegraphics[trim=140 50 400 60,clip,width=1.50in]{sections/figures/hmr_images/coco_gt/COCO_train2014_000000031335.jpg}};
  
  \node[picture format,anchor=north west]      (B2) at (A2.north east) {\includegraphics[trim=140 50 400 60,clip,width=1.50in]{sections/figures/hmr_images/coco/COCO_train2014_000000031335_mesh_fit.png}};

  % \node[picture format,anchor=north west] (A3) at (A2.north east) {\includegraphics[trim=140 50 400 60,clip,width=.60in]{sections/figures/hmr_images/coco/COCO_train2014_000000031335_mesh_fit.png}};
  % \node[picture format,anchor=north]      (B3) at (A3.south)      {\includegraphics[trim=0 90 200 100,clip,width=.75in]{sections/figures/hmr_images/coco/COCO_train2014_000000273665_mesh_fit.png}};
  %   \node[picture format,anchor=north]      (C3) at (B3.south)      {\includegraphics[trim=400 0 0 0,clip,width=.65in]{sections/figures/hmr_images/coco/COCO_train2014_000000175669_mesh_fit.png}};
  %     \node[picture format,anchor=north]      (D3) at (C3.south)      {\includegraphics[trim=100 100 400 100,clip,width=0.7in]{sections/figures/hmr_images/coco/COCO_train2014_000000525169_mesh_fit.png}};

  %% Captions

  % \node[anchor=south] (E2) at (A2.north) {\bfseries 3DPW\cite{vonMarcard2018}};
  % \node[anchor=south] (E3) at (A3.north) {\bfseries COCO\cite{lin2014microsoft}};

\end{tikzpicture}
\caption{Qualitative Results from \method{} for 3D pose estimation across the EHF\cite{SMPL-X:2019}, 3DPW\cite{vonMarcard2018}, and COCO\cite{lin2014microsoft} Original vs Predicted (3)} 
\label{fig:qual_hmr_vs_ori_1}
\end{figure}

\begin{figure}
\centering
\begin{tikzpicture}[picture format/.style={inner sep=1pt, outer sep=0pt}]

  \node[picture format]                   (A1)               {\includegraphics[trim=0 90 200 100,clip,width=1.75in]{sections/figures/hmr_images/coco_gt/COCO_train2014_000000273665.jpg}};
  
  \node[picture format,anchor=north west]      (B1) at (A1.north east)  {\includegraphics[trim=0 90 200 100,clip,width=1.75in]{sections/figures/hmr_images/coco/COCO_train2014_000000273665_mesh_fit.png}};
\node[anchor=south] (C1) at (A1.north) {\bfseries Original};
\node[anchor=south] (C2) at (B1.north) {\bfseries \method{}(Ours)};

  \node[picture format, anchor=north] (A2) at (A1.south)     {\includegraphics[trim=400 0 0 0,clip,width=1.65in]{sections/figures/hmr_images/coco_gt/COCO_train2014_000000175669.jpg}};
  
  \node[picture format,anchor=north west]      (B2) at (A2.north east) {\includegraphics[trim=400 0 0 0,clip,width=1.65in]{sections/figures/hmr_images/coco/COCO_train2014_000000175669_mesh_fit.png}};

  % \node[picture format,anchor=north west] (A3) at (A2.north east) {\includegraphics[trim=140 50 400 60,clip,width=.60in]{sections/figures/hmr_images/coco/COCO_train2014_000000031335_mesh_fit.png}};
  % \node[picture format,anchor=north]      (B3) at (A3.south)      {\includegraphics[trim=0 90 200 100,clip,width=.75in]{sections/figures/hmr_images/coco/COCO_train2014_000000273665_mesh_fit.png}};
  %   \node[picture format,anchor=north]      (C3) at (B3.south)      {\includegraphics[trim=400 0 0 0,clip,width=.65in]{sections/figures/hmr_images/coco/COCO_train2014_000000175669_mesh_fit.png}};
  %     \node[picture format,anchor=north]      (D3) at (C3.south)      {\includegraphics[trim=100 100 400 100,clip,width=0.7in]{sections/figures/hmr_images/coco/COCO_train2014_000000525169_mesh_fit.png}};

  %% Captions

  % \node[anchor=south] (E2) at (A2.north) {\bfseries 3DPW\cite{vonMarcard2018}};
  % \node[anchor=south] (E3) at (A3.north) {\bfseries COCO\cite{lin2014microsoft}};

\end{tikzpicture}
\caption{Qualitative Results from \method{} for 3D pose estimation across the EHF\cite{SMPL-X:2019}, 3DPW\cite{vonMarcard2018}, and COCO\cite{lin2014microsoft} Original vs Predicted (4)} 
\label{fig:qual_hmr_vs_ori_1}
\end{figure}

\begin{figure}
\centering
\begin{tikzpicture}[picture format/.style={inner sep=15pt, outer sep=0pt}]

  \node[picture format]                   (A1)               {\includegraphics[width=3.75in]{sections/figures/hmr_images/coco_gt/COCO_train2014_000000525169.jpg}};
  
  \node[picture format,anchor=north]      (B1) at (A1.south)  {\includegraphics[width=3.75in]{sections/figures/hmr_images/coco/COCO_train2014_000000525169_mesh_fit.png}};
\node[anchor=south] (C1) at (A1.north) {\bfseries Original};
\node[anchor=south] (C2) at (B1.north) {\bfseries \method{}(Ours)};

  % \node[picture format,anchor=north west] (A3) at (A2.north east) {\includegraphics[trim=140 50 400 60,clip,width=.60in]{sections/figures/hmr_images/coco/COCO_train2014_000000031335_mesh_fit.png}};
  % \node[picture format,anchor=north]      (B3) at (A3.south)      {\includegraphics[trim=0 90 200 100,clip,width=.75in]{sections/figures/hmr_images/coco/COCO_train2014_000000273665_mesh_fit.png}};
  %   \node[picture format,anchor=north]      (C3) at (B3.south)      {\includegraphics[trim=400 0 0 0,clip,width=.65in]{sections/figures/hmr_images/coco/COCO_train2014_000000175669_mesh_fit.png}};
  %     \node[picture format,anchor=north]      (D3) at (C3.south)      {\includegraphics[trim=100 100 400 100,clip,width=0.7in]{sections/figures/hmr_images/coco/COCO_train2014_000000525169_mesh_fit.png}};

  %% Captions

  % \node[anchor=south] (E2) at (A2.north) {\bfseries 3DPW\cite{vonMarcard2018}};
  % \node[anchor=south] (E3) at (A3.north) {\bfseries COCO\cite{lin2014microsoft}};

\end{tikzpicture}
\caption{Qualitative Results from \method{} for 3D pose estimation across the EHF\cite{SMPL-X:2019}, 3DPW\cite{vonMarcard2018}, and COCO\cite{lin2014microsoft} Original vs Predicted (5)} 
\label{fig:qual_hmr_vs_ori_1}
\end{figure}

\newpage

\begin{table}[!t]
\centering
\setlength{\tabcolsep}{1mm}
\begin{tabular}{lcc}
\toprule
\textbf{Method}                     & $\Delta\textbf{q}+\text{m2m}\downarrow$ & $\text{m2m}(\text{cm})\downarrow$   \\
\midrule
PoseNDF\cite{tiwari2022pose}    & - & - \\
NRDF\cite{he2024nrdf}           & 0.313 & 24.93 \\
DPoser\cite{lu2023dposer}          & - & - \\
% \method{} (Ours, $t=1000, \Delta 5$)                & 0.093 & 8.58 \\
% \method{} (Ours, $t=900, \Delta 5$)                & 0.301 & 23.60 \\
\method{} (Ours, $t=900, \Delta 5$)                & 0.322 & 24.93 \\
% \method{} (Ours, $t=900, \Delta 10$)                & 0.075 & 7.01 \\
% \method{} (Ours, $t=900, \Delta 5$)                & 0.084 & 7.84 \\
% \method{} (Ours, $t=900, \Delta 2$)                & 0.109 & 9.95 \\
% \method{} (Ours, $t=400, \Delta 5$)                & 0.133 & 11.72 \\
% \method{} (Ours, $t=400, \Delta 2$)               & 0.146 & 12.81\\
% \method{} (Ours, $t=200, \Delta 2$)               & 0.207 & 17.05\\
\bottomrule
\end{tabular}
\label{Table:denoise}
\caption{TODO:regenerate noisy poses. Comparison with baseline methods for pose denoising. m2m is reported in centimeters. Testing other choices in time-steps scheduling show that choosing the right start step is critical. Consistency models\cite{song2023consistency} and other alternatives may be able to help remove the need to choose the optimal parameters.} 
\end{table}
\subsection{Pose Denoising}
In line with previous works we demonstrate \method{}'s effectiveness on the task of pose denoising. For this experiment we follow the experiment outlined in NRDF\cite{he2024nrdf} and report the $\Delta\textbf{q} + \text{m2m}$ and m2m metrics. The $\Delta\textbf{q}$ metric is defined as the quaternion geodesic distance in the global frame and the Euclidean marker to marker distance $\text{m2m}$ which \cite{he2024nrdf} shows in user-studies is correlated to human preference over other metrics. The noisy samples are sampled from the AMASS test split and noisy poses are generated using the procedure outlined in NRDF. For the denoising task we simply employ DDIM based sampling where we start at $t=400$ with a step size of $5$ which is empirically chosen. This is in contrast to the optimization based framework adopted by other pose priors such as PoseNDF\cite{tiwari2022pose} or NRDF where DDIM sampling is computationally cheaper as we do not need to back-propagate through the network. For 100 poses it takes NRDF $2.1$ seconds while it takes \method{} $0.83$ seconds for the same input using an RTX A5000. Overall, we can see that \method{} demonstrates superior performance over all other pose priors.
